# Supplementary material for: Theories of "Gender" in NLP Bias Research
Source: arXiv:2205.02526 source file (2022-05-05)
Supplement: Supplementary file 1 [file appendix_bib.pdf]

## A FULL BIBLIOGRAPHY OF SURVEYED PAPERS

### REFERENCES

- [1] Gavin Abercrombie, Amanda Cercas Curry, Mugdha Pandya, and Verena Rieser. 2021. Alexa, Google, Siri: What are Your Pronouns? Gender and Anthropomorphism in the Design and Perception of Conversational Assistants. In *Proceedings of the 3rd Workshop on Gender Bias in Natural Language Processing*. Association for Computational Linguistics (ACL), Online, 24–33. <https://doi.org/10.18653/V1/2021.GEBNLP-1.4>
- [2] Artem Abzaliev. 2019. On GAP coreference resolution shared task: insights from the 3rd place solution. In *Proceedings of the First Workshop on Gender Bias in Natural Language Processing*. Association for Computational Linguistics, Florence, Italy, 107–112. <https://doi.org/10.18653/v1/W19-3816>
- [3] Felipe Alfaro, Lois José, A R Fonollosa, and Marta R Costa-Jussà. 2019. BERT Masked Language Modeling for Co-reference Resolution. In *Proceedings of the First Workshop on Gender Bias in Natural Language Processing*. Association for Computational Linguistics, Florence, Italy, 76–81. <https://doi.org/10.18653/v1/W19-3811>
- [4] Ananya, Nitya Parthasarathi, and Sameer Singh. 2019. GenderQuant: Quantifying Mention-Level Genderedness. In *Proceedings of the 2019 Conference of the North American Chapter of the Association for Computational Linguistics: Human Language Technologies, Volume 1 (Long and Short Papers)*. Association for Computational Linguistics, Minneapolis, Minnesota, 2959–2969. <https://doi.org/10.18653/V1/N19-1303>
- [5] Sandeep Attree. 2019. Gendered Ambiguous Pronouns Shared Task: Boosting Model Confidence by Evidence Pooling. In *Proceedings of the First Workshop on Gender Bias in Natural Language Processing*. Association for Computational Linguistics, Florence, Italy, 134–146. <https://doi.org/10.18653/v1/W19-3820>
- [6] Marzieh Babaeianjelodar, Stephen Lorenz, Josh Gordon, Jeanna Matthews, and Evan Freitag. 2020. Quantifying Gender Bias in Different Corpora | Enhanced Reader.pdf. In *Companion Proceedings of the Web Conference 2020 (WWW’20 Companion)*. ACM, New York, New York, USA, 752–759. <https://dl.acm-org.proxy.ub.umu.se/doi/abs/10.1145/3366424.3383559>
- [7] David Bamman, Sejal Popat, and Sheng Shen. 2019. An Annotated Dataset of Literary Entities. In *Proceedings of the 2019 Conference of the North American Chapter of the Association for Computational Linguistics: Human Language Technologies*. Association for Computational Linguistics, Minneapolis, Minnesota, 2138–2144. <https://doi.org/10.18653/v1/N19-1220>
- [8] Xingce Bao and Qianqian Qiao. 2019. Transfer Learning from Pre-trained BERT for Pronoun Resolution. In *Proceedings of the First Workshop on Gender Bias in Natural Language Processing*. Association for Computational Linguistics, Florence, Italy, 82–88. <https://doi.org/10.18653/v1/W19-3812>
- [9] Marion Bartl, Malvina Nissim, and Albert Gatt. 2020. Unmasking Contextual Stereotypes: Measuring and Mitigating BERT’s Gender Bias. In *Proceedings of the Second Workshop on Gender Bias in Natural Language Processing*. Association for Computational Linguistics, Barcelona, Spain (Online), 1–16. <https://aclanthology.org/2020.gebnlp-1.1>
- [10] Christine Basta, Marta R Costa-Jussà, and Noe Casas. 2019. Evaluating the Underlying Gender Bias in Contextualized Word Embeddings. In *Proceedings of the First Workshop on Gender Bias in Natural Language Processing*. Association for Computational Linguistics, Florence, Italy, 33–39. <https://doi.org/10.18653/v1/W19-3805>
- [11] Christine Basta, Marta R Costa-Jussà, and • Noe Casas. 2020. Extensive study on the underlying gender bias in contextualized word embeddings. *Neural Computing and Applications* 33 (2020), 3371–3384. <https://doi.org/10.1007/s00521-020-05211-z>
- [12] Christine Raouf Saad Basta, Marta Ruiz Costa-Jussà, and José Adrián Rodríguez Fonollosa. 2020. Towards mitigating gender bias in a decoder-based neural machine translation model by adding contextual information. In *Proceedings of the The Fourth Widening Natural Language Processing Workshop*. Association for Computational Linguistics, Seattle, USA, 99–102. <https://doi.org/10.18653/V1/2020.WINLP-1.25>
- [13] Rishabh Bhardwaj, Navonil Majumder, and Soujanya Poria. 2021. Investigating Gender Bias in BERT. *Cognitive Computation* 13 (2021), 1008–1018. <https://doi.org/10.1007/s12559-021-09881-2>
- [14] Shruti Bhargava and David Forsyth. 2019. *Exposing and Correcting the Gender Bias in Image Captioning Datasets and Models*. Technical Report. University of Illinois at Urbana-Champaign. arXiv:1912.00578 <http://arxiv.org/abs/1912.00578>
- [15] Jayadev Bhaskaran and Isha Bhallamudi. 2019. Good Secretaries, Bad Truck Drivers? Occupational Gender Stereotypes in Sentiment Analysis. In *Proceedings of the First Workshop on Gender Bias in Natural Language Processing*. Association for Computational Linguistics, Florence, Italy, 62–68. <https://doi.org/10.18653/v1/W19-3809>
- [16] Tolga Bolukbasi, Kai Wei Chang, James Zou, Venkatesh Saligrama, and Adam Kalai. 2016. Man is to computer programmer as woman is to homemaker? Debiasing word embeddings. In *Advances in Neural Information Processing Systems*. NeurIPS, Barcelona, Spain, 4356–4364. arXiv:1607.06520 <http://papers.nips.cc/paper/6228-man-is-to-computer-programmer-as-woman-is-to-homemaker-d>
- [17] Tolga Bolukbasi, Kai-Wei Chang, James Zou, Venkatesh Saligrama, and Adam Kalai. 2016. Quantifying and Reducing Stereotypes in Word Embeddings. In *ICML Workshop on #Data4Good: Machine Learning in Social Good Applications*. ICML, New York, New York, USA, 41–45. arXiv:1606.06121 <http://arxiv.org/abs/1606.06121>
- [18] Shikha Bordia and Samuel R. Bowman. 2019. Identifying and Reducing Gender Bias in Word-Level Language Models. In *Proceedings of the 2019 Conference of the North American Chapter of the Association for Computational Linguistics: Student Research Workshop*. Association for Computational Linguistics, Minneapolis, Minnesota, 7–15. <https://doi.org/10.18653/v1/N19-3002> arXiv:1904.03035
- [19] Clothilde Breger, Ghasem Elyasi, Guillermo Infante, and Mariano Zarza. 2020. Reducing Gender Bias in Natural Language Processing methods. In *Meta Research Research Methods Course: Master in Intelligent and Interactive Systems*, Davinia Hernández-Leo and Judit Martínez-Moreno (Eds.). Universitat Pompeu Fabra, Barcelona, Spain, 17–24. <http://repositori.upf.edu/>

- [20] Marc-Etienne Brunet, Colleen Alkalay-Houlihan, Ashton Anderson, and Richard Zemel. 2019. Understanding the origins of bias in word embeddings. In *36th International Conference on Machine Learning*, Vol. 97. Proceedings of Machine Learning Research, Irvine, CA, USA, 803–811. arXiv:1810.03611 <http://proceedings.mlr.press/v97/brunet19a.html>
- [21] Kaylee Burns, Lisa Anne Hendricks, Kate Saenko, Trevor Darrell, and Anna Rohrbach. 2018. Women also Snowboard: Overcoming Bias in Captioning Models. In *Proceedings of the European Conference on Computer Vision*. ECCV, Munich, Germany, 771–787. arXiv:1803.09797 <http://arxiv.org/abs/1803.09797>
- [22] Aylin Caliskan, Joanna J Bryson, and Arvind Narayanan. 2017. Semantics derived automatically from language corpora contain human-like biases. *Science (New York, N.Y.)* 356, 6334 (apr 2017), 183–186. <https://doi.org/10.1126/science.aal4230>
- [23] Yang Trista Cao and Hal Daumé III. 2020. Toward Gender-Inclusive Coreference Resolution. In *Proceedings of the 58th Annual Meeting of the Association for Computational Linguistics*. Association for Computational Linguistics, Online, 4568–4595. <https://doi.org/10.18653/v1/2020-acl-main.418>
- [24] Rakesh Chada. 2019. Gendered Pronoun Resolution using BERT and an extractive question answering formulation. In *Proceedings of the First Workshop on Gender Bias in Natural Language Processing*. Association for Computational Linguistics, Florence, Italy, 126–133. <https://doi.org/10.18653/v1/W19-3819>
- [25] Kaytlin Chaloner and Alfredo Maldonado. 2019. Measuring Gender Bias in Word Embeddings across Domains and Discovering New Gender Bias Word Categories. In *Proceedings of the First Workshop on Gender Bias in Natural Language Processing*. Association for Computational Linguistics, Florence, Italy, 25–32. <https://doi.org/10.18653/v1/W19-3804>
- [26] Serina Chang and Kathleen McKeown. 2019. Automatically Inferring Gender Associations from Language. In *Conference on Empirical Methods in Natural Language Processing*. Association for Computational Linguistics, Hong Kong, 5746–5752. <https://doi.org/10.18653/v1/D19-1579>
- [27] Yan Chen, Christopher Mahoney, Isabella Grasso, Esma Wali, Abigail Matthews, Thomas Middleton, Mariama Njie, and Jeanna Matthews. 2021. Gender Bias and Under-Representation in Natural Language Processing Across Human Languages; Gender Bias and Under-Representation in Natural Language Processing Across Human Languages. In *Proceedings of the 2021 AAAI/ACM Conference on AI, Ethics, and Society (AIES '21)*. Association for Computing Machinery, Virtual Event, 11 pages. <https://doi.org/10.1145/3461702.3462530>
- [28] Won Ik Cho, Ji Won Kim, Min Kim, and Nam Soo Kim. 2019. On Measuring Gender Bias in Translation of Gender-neutral Pronouns. In *Proceedings of the First Workshop on Gender Bias in Natural Language Processing*. Association for Computational Linguistics, Florence, Italy, 173–181. <https://doi.org/10.18653/v1/W19-3824>
- [29] Shivang Chopra, Ramit Sawhney, Puneet Mathur, and Rajiv Ratn Shah. 2020. Hindi-English Hate Speech Detection: Author Profiling, Debiasing, and Practical Perspectives. In *Proceedings of the AAAI Conference on Artificial Intelligence*, Vol. 34. Association for the Advancement of Artificial Intelligence (AAAI), New York, NY, USA, 386–393. <https://doi.org/10.1609/aaai.v34i01.5374>
- [30] Marta R Costa-Jussà. 2019. An analysis of gender bias studies in natural language processing. *Nature Machine Intelligence* 1, 11 (2019), 495–496. <https://doi.org/10.1038/s42256-019-0105-5>
- [31] Marta R. Costa-jussà and Adrià de Jorge. 2020. Fine-tuning Neural Machine Translation on Gender-Balanced Datasets. In *Proceedings of the Second Workshop on Gender Bias in Natural Language Processing*. Association for Computational Linguistics, Barcelona, Spain, 26–34. <https://aclanthology.org/2020.gebnlp-1.3>
- [32] Marta R. Costa-jussà, Carlos Escolano, Christine Basta, Javier Ferrando, Roser Batlle, and Ksenia Kharitonova. 2020. *Gender Bias in Multilingual Neural Machine Translation: The Architecture Matters*. Technical Report. TALP Research Center, Universitat Politècnica de Catalunya, Barcelona. arXiv:2012.13176 <https://arxiv.org/abs/2012.13176>
- [33] Amanda Cercas Curry and Verena Rieser. 2018. #MeToo: How Conversational Systems Respond to Sexual Harassment. In *Proceedings of the Second ACL Workshop on Ethics in Natural Language Processing*. Association for Computational Linguistics, New Orleans, Louisiana, USA, 7–14. <https://doi.org/10.18653/v1/W18-0802>
- [34] Karan Dabas, Nishtha Madan, Vijay Arya, Sameep Mehta, Gautam Singh, and Tanmoy Chakraborty. 2019. Fair Transfer of Multiple Style Attributes in Text. In *2019 Grace Hopper Celebration India, GHCI*. IEEE, Bangalore, India, 1–5. <https://doi.org/10.1109/GHCI47972.2019.9071799> arXiv:2001.06693
- [35] Jamell Dacon and Haochen Liu. 2021. Does Gender Matter in the News? Detecting and Examining Gender Bias in News Articles. In *The Web Conference 2021 - Companion of the World Wide Web Conference, WWW 2021*, Vol. 2. Association for Computing Machinery, Ljubljana, Slovenia, 385–392. <https://doi.org/10.1145/3442442.3452325>
- [36] Erenay Dayanik and Sebastian Padó. 2021. Disentangling Document Topic and Author Gender in Multiple Languages: Lessons for Adversarial Debiasing. In *Proceedings of the Eleventh Workshop on Computational Approaches to Subjectivity, Sentiment and Social Media Analysis*. Association for Computational Linguistics, Online, 50–61. <https://aclanthology.org/2021.wassa-1.6>
- [37] Maria De-Arteaga, Alexey Romanov, Hanna Wallach, Jennifer Chayes, Christian Borgs, Alexandra Chouldechova, Sahin Geyik, Krishnaram Kenthapadi, and Adam Tauman Kalai. 2019. Bias in Bios: A Case Study of Semantic Representation Bias in a High-Stakes Setting. In *Proceedings of the Conference on Fairness, Accountability, and Transparency*. Association for Computing Machinery, Atlanta, Georgia, USA, 120–128. <https://doi.org/10.1145/3287560.3287572>
- [38] Sunipa Dev, Tao Li, Jeff Phillips, and Vivek Srikumar. 2020. On Measuring and Mitigating Biased Inferences of Word Embeddings. In *Proceedings of the AAAI Conference on Artificial Intelligence*. AAAI press, New York, NY, USA, 7659–7666. <https://doi.org/10.1609/aaai.v34i05.6267>

- [39] Sunipa Dev and Jeff Phillips. 2019. Attenuating Bias in Word Vectors. In *AISTATS 2019 - 22nd International Conference on Artificial Intelligence and Statistics*. PLMR, Naha, Okinawa, Japan, 879–887. arXiv:1901.07656 <http://proceedings.mlr.press/v89/dev19a.html>
- [40] Emily Dinan, Angela Fan, Adina Williams, Jack Urbanek, Douwe Kiela, and Jason Weston. 2020. Queens are powerful too: Mitigating gender bias in dialogue generation. In *Proceedings of the 2020 Conference on Empirical Methods in Natural Language Processing (EMNLP)*. Association for Computational Linguistics, Online, 8173–8188. <https://doi.org/10.18653/v1/2020.emnlp-main.656>
- [41] Emily Dinan, Angela Fan, Ledell Wu, Jason Weston, Douwe Kiela, and Adina Williams. 2020. Multi-Dimensional Gender Bias Classification. In *Proceedings of the 2020 Conference on Empirical Methods in Natural Language Processing (EMNLP)*. Association for Computational Linguistics, Online, 314–331. <https://doi.org/10.18653/v1/2020.emnlp-main.23>
- [42] Jad Doughman, Wael Khreich, Maya El Gharib, Maha Wiss, and Zahraa Berjawi. 2021. Gender Bias in Text: Origin, Taxonomy, and Implications. In *Proceedings of the 3rd Workshop on Gender Bias in Natural Language Processing*. Association for Computational Linguistics (ACL), Online, 34–44. <https://doi.org/10.18653/V1/2021.GEBNLP-1.5>
- [43] Yupei Du, Yuanbin Wu, and Man Lan. 2019. Exploring Human Gender Stereotypes with Word Association Test. In *Proceedings of the 2019 Conference on Empirical Methods in Natural Language Processing and the 9th International Conference on Natural Language Processing*. Association for Computational Linguistics, Hong Kong, 6133–6143. <https://doi.org/10.18653/v1/D19-1635>
- [44] Ali Emami, Paul Trichelair, Adam Trischler, Kaheer Suleman, Hannes Schulz, Jackie Chi, and Kit Cheung. 2019. The KNOWREF Coreference Corpus: Removing Gender and Number Cues for Difficult Pronominal Anaphora Resolution. In *Proceedings of the 57th Annual Meeting of the Association for Computational Linguistics*. Association for Computational Linguistics, Florence, Italy, 3952–3961. <https://doi.org/10.18653/v1/P19-1386>
- [45] Kawin Ethayarajh. 2020. Is Your Classifier Actually Biased? Measuring Fairness under Uncertainty with Bernstein Bounds. In *Proceedings of the 58th Annual Meeting of the Association for Computational Linguistics*. Association for Computational Linguistics, Online, 2914–2919. <https://doi.org/10.18653/v1/2020.acl-main.262> arXiv:2004.12332
- [46] Kawin Ethayarajh, David Duvenaud, and Graeme Hirst. 2019. Understanding undesirable word embedding associations. In *Proceedings of the 57th Annual Meeting of the Association for Computational Linguistics*. Association for Computational Linguistics, Florence, Italy, 1696–1705. <https://doi.org/10.18653/v1/P19-1166> arXiv:1908.06361
- [47] Joseph Fisher, Dave Palfrey, Christos Christodoulopoulos, and Arpit Mittal. 2020. Measuring Social Bias in Knowledge Graph Embeddings. In *Workshop on Bias in Automatic Knowledge Graph Construction (KG-BIAS)*. Automated Knowledge Base Construction, Online. arXiv:1912.02761 <http://arxiv.org/abs/1912.02761>
- [48] Eve Fleisig. 2021. *Adversarial Learning for Bias Mitigation in Machine Translation*. Bachelor of Science in Engineering. Princeton University.
- [49] Omar U. Florez. 2019. *On the Unintended Social Bias of Training Language Generation Models with Data from Local Media*. Technical Report. arXiv:1911.00461 <http://arxiv.org/abs/1911.00461>
- [50] Joel Escudé Font and Marta R Costa-Jussà. 2019. Equalizing Gender Bias in Neural Machine Translation with Word Embeddings Techniques. In *Proceedings of the First Workshop on Gender Bias in Natural Language Processing*. Association for Computational Linguistics, Florence, Italy, 147–154. <https://doi.org/10.18653/v1/W19-3821>
- [51] Nikhil Garg, Londa Schiebinger, Dan Jurafsky, and James Zou. 2018. Word embeddings quantify 100 years of gender and ethnic stereotypes. *Proceedings of the National Academy of Sciences of the United States of America* 115, 16 (apr 2018), E3635–E3644. <https://doi.org/10.1073/pnas.1720347115> arXiv:1711.08412
- [52] Aparna Garimella, Carmen Banea, Dirk Hovy, and Rada Mihalcea. 2019. Women’s syntactic resilience and men’s grammatical luck: Gender-bias in part-of-speech tagging and dependency parsing. In *Proceedings of the 57th Annual Meeting of the Association for Computational Linguistics*. Association for Computational Linguistics, Florence, Italy, 3493–3498. <https://doi.org/10.18653/v1/p19-1339>
- [53] Andrew Gaut, Tony Sun, Shirlyn Tang, Yuxin Huang, Jing Qian, Mai ElSherief, Jieyu Zhao, Diba Mirza, Elizabeth Belding, Kai-Wei Chang, and William Yang Wang. 2020. Towards Understanding Gender Bias in Relation Extraction. In *Proceedings of the 58th Annual Meeting of the Association for Computational Linguistics*. Association for Computational Linguistics, Online, 2943–2953. <https://doi.org/10.18653/v1/2020.acl-main.265> arXiv:1911.03642
- [54] Oguzhan Gencoglu. 2021. Cyberbullying Detection with Fairness Constraints. *IEEE Internet Computing* 25, 1 (may 2021), 20–29. <https://doi.org/10.1109/MIC.2020.3032461> arXiv:2005.06625
- [55] Seraphina Goldfarb-Tarrant, Rebecca Marchant, Ricardo Muñoz, Mu- Muñoz Sánchez, Mugdha Pandya, and Adam Lopez. 2021. Intrinsic Bias Metrics Do Not Correlate with Application Bias. In *Proceedings of the 59th Annual Meeting of the Association for Computational Linguistics and the 11th International Joint Conference on Natural Language Processing*. Association for Computational Linguistics (ACL), 1926–1940. <https://doi.org/10.18653/v1/2021.acl-long.150> arXiv:2012.15859
- [56] Hila Gonen and Yoav Goldberg. 2019. Lipstick on a Pig: Debiasing Methods Cover up Systematic Gender Biases in Word Embeddings But do not Remove Them. In *Proceedings of the 2019 Conference of the North American Chapter of the Association for Computational Linguistics: Human Language Technologies*. Association for Computational Linguistics, Minneapolis, Minnesota, 609–614. <https://doi.org/10.18653/v1/N19-1061> arXiv:1903.03862
- [57] Hila Gonen and Kellie Webster. 2020. Automatically Identifying Gender Issues in Machine Translation using Perturbations. In *Findings of the Association for Computational Linguistics: EMNLP 2020*. Association for Computational Linguistics (ACL), 1991–1995. <https://doi.org/10.18653/v1/2020.findings-emnlp.180> arXiv:2004.14065
- [58] Nizar Habash, Houda Bouamor, and Christine Chung. 2019. Automatic Gender Identification and Reinflection in Arabic. In *Proceedings of the First Workshop on Gender Bias in Natural Language Processing*. Association for Computational Linguistics, Florence, Italy, 155–165. <https://doi.org/10.18653/v1/2019.gbnlp.1>

- [//doi.org/10.18653/v1/W19-3822](https://doi.org/10.18653/v1/W19-3822)
- [59] Saga Hansson, Konstantinos Mavromatakis, Yvonne Adesam, Gerlof Bouma, and Dana Dannélls. 2021. The Swedish Winogender Dataset. In *Proceedings of the 23rd Nordic Conference on Computational Linguistics (NoDaLiDa)*. Linköping University Electronic Press, Sweden, Reykjavik, Iceland (Online), 452–459. <https://aclanthology.org/2021.nodalida-main.52>
  - [60] Reyhane Hashempour, Aline Villavicencio, Barbara Plank, and Renato Amorim. 2019. A Deep Learning Approach to Language-independent Gender Prediction on Twitter. In *Proceedings of the 2019 Workshop on Widening NLP*. <https://doi.org/10.1016/j.diin.2011.04.002>
  - [61] Dirk Hovy, Federico Bianchi, and Tommaso Fornaciari. 2020. *Can You Translate that into Man? Commercial Machine Translation Systems Include Stylistic Biases*. Technical Report. <https://www.cia.gov/library/>
  - [62] Alexander Hoyle, Wolf-Sonkin, Hanna Wallach, Isabelle Augenstein, and Ryan Cotterell. 2019. Unsupervised Discovery of Gendered Language through Latent-Variable Modeling. In *Proceedings of the 57th Annual Meeting of the Association for Computational Linguistics*. Association for Computational Linguistics, 1706–1716. <https://doi.org/10.18653/v1/P19-1167> arXiv:1906.04760
  - [63] Po-Sen Huang, Huan Zhang, Ray Jiang, Robert Stanforth, Johannes Welbl, Jack Rae, Vishal Maini, Dani Yogatama, and Pushmeet Kohli. 2020. Reducing Sentiment Bias in Language Models via Counterfactual Evaluation. In *Findings of the Association for Computational Linguistics: EMNLP 2020*. Association for Computational Linguistics, 65–83. <https://doi.org/10.18653/v1/2020.findings-emnlp.7> arXiv:1911.03064
  - [64] Xiaolei Huang, Linzi Xing, Franck Dernoncourt, and Michael J. Paul. 2020. Multilingual Twitter Corpus and Baselines for Evaluating Demographic Bias in Hate Speech Recognition. In *Proceedings of the 12th Conference on Language Resources and Evaluation (LREC 2020)*. European Language Resources Association (ELRA), Marseille, France, 1440–1448. arXiv:2002.10361 <http://www.lrec-conf.org/proceedings/lrec2020/pdf/2020.lrec-1.180.pdf>
  - [65] Matei Ionita, Yury Kashnitsky, Ken Krige Kitsong, Vladimir Larin, Pjsc Sberbank, Denis Logvinenko, and Atanas Atanasov. 2019. Resolving Gendered Ambiguous Pronouns with BERT. In *Proceedings of the First Workshop on Gender Bias in Natural Language Processing*. Association for Computational Linguistics, Florence, Italy, 113–119. <https://doi.org/10.18653/v1/W19-3817>
  - [66] Nishtha Jain, Maja Popović, Declan Groves, and Eva Vanmassenhove. 2021. Generating Gender Augmented Data for NLP. In *Proceedings of the 3rd Workshop on Gender Bias in Natural Language Processing*. Association for Computational Linguistics (ACL), Online, 93–102. <https://doi.org/10.18653/V1/2021.GEBNLP-1.11>
  - [67] Hailey James and David Alvarez-Melis. 2019. Probabilistic Bias Mitigation in Word Embeddings. In *Human-Centric Machine Learning Workshop, NeurIPS 2019*. arXiv:1910.14497 <http://arxiv.org/abs/1910.14497>
  - [68] Shengyu Jia, Tao Meng, Jieyu Zhao, and Kai-Wei Chang. 2020. Mitigating Gender Bias Amplification in Distribution by Posterior Regularization. In *Proceedings of the 58th Annual Meeting of the Association for Computational Linguistics*. Association for Computational Linguistics, Online, 2936–2942. <https://doi.org/10.18653/v1/2020.acl-main.264> arXiv:2005.06251
  - [69] May Jiang and Christiane Fellbaum. 2020. Interdependencies of Gender and Race in Contextualized Word Embeddings. In *Proceedings of the Second Workshop on Gender Bias in Natural Language Processing*. Barcelona, Spain (Online), 17–25. <https://aclanthology.org/2020.gebnlp-1.2>
  - [70] Meichun Jiao and Ziyang Luo. 2021. Gender Bias Hidden Behind Chinese Word Embeddings: The Case of Chinese Adjectives. In *Proceedings of the Second Workshop on Gender Bias in Natural Language Processing*. Association for Computational Linguistics (ACL), Barcelona, Spain (Online), 8–15. <https://doi.org/10.18653/V1/2021.GEBNLP-1.2>
  - [71] Jaap Jumelet, Willem Zuidema, and Dieuwke Hupkes. 2019. Analysing Neural Language Models: Contextual Decomposition Reveals Default Reasoning in Number and Gender Assignment. In *CoNLL 2019 - 23rd Conference on Computational Natural Language Learning, Proceedings of the Conference*. Association for Computational Linguistics, Hong Kong, 1–11. <https://doi.org/10.18653/v1/K19-1001> arXiv:1909.08975
  - [72] Masahiro Kaneko and Danushka Bollegala. 2019. Gender-preserving Debiasing for Pre-trained Word Embeddings. In *Proceedings of the 57th Annual Meeting of the Association for Computational Linguistics*. Association for Computational Linguistics (ACL), Florence, Italy, 1641–1650. <https://doi.org/10.18653/v1/P19-1160> arXiv:1906.00742
  - [73] Masahiro Kaneko and Danushka Bollegala. 2021. Dictionary-based Debiasing of Pre-trained Word Embeddings. In *Proceedings of the 16th Conference of the European Chapter of the Association for Computational Linguistics: Main Volume*. Association for Computational Linguistics, Online, 212–223. <https://aclanthology.org/2021.eacl-main.16>
  - [74] Dongyeop Kang, Varun Gangal, and Eduard Hovy. 2019. (Male, Bachelor) and (Female, Ph.D) have different connotations: Parallely Annotated Stylistic Language Dataset with Multiple Personas. In *Proceedings of the 2019 Conference on Empirical Methods in Natural Language Processing and the 9th International Joint Conference on Natural Language Processing (EMNLP-IJCNLP)*. Association for Computational Linguistics, Hong Kong, 1696–1706. <https://www.aclweb.org/anthology/D19-1179/>
  - [75] Saket Karve, Lyle Ungar, and João Sedoc. 2019. Conceptor Debiasing of Word Representations Evaluated on WEAT. (jun 2019), 40–48. arXiv:1906.05993 <http://arxiv.org/abs/1906.05993>
  - [76] Jae Yeon Kim, Carlos Ortiz, Sarah Nam, Sarah Santiago, and Vivek Datta. 2020. Intersectional Bias in Hate Speech and Abusive Language Datasets. (may 2020). arXiv:2005.05921 <http://arxiv.org/abs/2005.05921>
  - [77] Svetlana Kiritchenko and Saif M. Mohammad. 2018. Examining Gender and Race Bias in Two Hundred Sentiment Analysis Systems. In *Proceedings of the Seventh Joint Conference on Lexical and Computational Semantics*. Association for Computational Linguistics, New Orleans, Louisiana, USA, 43–53. <https://www.aclweb.org/anthology/S18-2005/>
  - [78] Vid Kocijan, Oana-Maria Camburu, and Thomas Lukasiewicz. 2020. The Gap on GAP: Tackling the Problem of Differing Data Distributions in Bias-Measuring Datasets. In *Proceedings of the 35th AAAI Conference on Artificial Intelligence, AAAI 2021*. AAAI, Online, 9727–9736. arXiv:2011.01837

- <https://arxiv.org/abs/2011.01837v3>
- [79] Vaibhav Kumar, Tenzin Singhay Bhotia, and Vaibhav Kumar. 2020. Fair Embedding Engine: A Library for Analyzing and Mitigating Gender Bias in Word Embeddings. In *Proceedings of Second Workshop for NLP Open Source Software (NLP-OSS)*. Association for Computational Linguistics (ACL), 26–31. <https://doi.org/10.18653/v1/2020.nlp-oss-1.5> arXiv:2010.13168
  - [80] Keita Kurita, Nidhi Vyas, Ayush Pareek, Alan W Black, and Yulia Tsvetkov. 2019. Measuring Bias in Contextualized Word Representations. (jun 2019), 166–172. arXiv:1906.07337 <http://arxiv.org/abs/1906.07337>
  - [81] Anne Lauscher and Goran Glavaš. 2019. Are We Consistently Biased? Multidimensional Analysis of Biases in Distributional Word Vectors. (apr 2019), 85–91. arXiv:1904.11783 <http://arxiv.org/abs/1904.11783>
  - [82] Anne Lauscher, Goran Glavaš, Simone Paolo Ponzetto, and Ivan Vulić. 2020. *A General Framework for Implicit and Explicit Debiasing of Distributional Word Vector Spaces*. Technical Report. [www.aaii.org](http://www.aaii.org)
  - [83] Nayeon Lee, Yejin Bang, Jamin Shin, and Pascale Fung. 2019. Understanding the Shades of Sexism in Popular TV Series. In *Proceedings of the 2019 Workshop on Widening NLP*. 177–180. <https://tv-tropes.org/>
  - [84] Nayeon Lee, Andrea Madotto, and Pascale Fung. 2019. Exploring Social Bias in Chatbots using Stereotype Knowledge. In *Proceedings of the Workshop on Widening NLP*. Florence, Italy, 177–180.
  - [85] Paul Pu Liang, Irene Li, Emily Zheng, Yao Chong Lim, Ruslan Salakhutdinov, and Louis-Philippe Morency. 2019. Towards Debiasing Sentence Representations. In *Proceedings of the NeurIPS Workshop on Human-Centric Machine Learning*. Vancouver, Canada.
  - [86] Bo Liu. 2019. *Anonymized BERT: An Augmentation Approach to the Gendered Pronoun Resolution Challenge*. Technical Report. 120–125 pages. <https://github.com/boliu61/gendered-pronoun-resolution>
  - [87] Haochen Liu, Jamell Dacon, Wenqi Fan, Hui Liu, Zitao Liu, and Jiliang Tang. 2019. Does Gender Matter? Towards Fairness in Dialogue Systems. (oct 2019). arXiv:1910.10486 <http://arxiv.org/abs/1910.10486>
  - [88] Kaiji Lu, Piotr Mardziel, Fangjing Wu, Preetam Amancharla, and Anupam Datta. 2020. Gender Bias in Neural Natural Language Processing. In *Logic, Language, and Security*. Springer International Publishing, Cham, 189–202. [https://doi.org/10.1007/978-3-030-62077-6\\_14](https://doi.org/10.1007/978-3-030-62077-6_14)
  - [89] Li Lucy and David Bamman. 2021. Gender and Representation Bias in GPT-3 Generated Stories. In *Proceedings of the Third Workshop on Narrative Understanding*. Association for Computational Linguistics (ACL), Virtual, 48–55. <https://doi.org/10.18653/v1/2021.NUSE-1.5>
  - [90] Thomas Manzini, Yao Chong Lim, Yulia Tsvetkov, and Alan W. Black. 2019. Black is to criminal as caucasian is to police: Detecting and removing multiclass bias in word embeddings. *NAACL HLT 2019 - 2019 Conference of the North American Chapter of the Association for Computational Linguistics: Human Language Technologies - Proceedings of the Conference 1* (apr 2019), 615–621. <https://doi.org/10.18653/v1/n19-1062> arXiv:1904.04047
  - [91] Abigail Matthews, Isabella Grasso, Christopher Mahoney, Yan Chen, Esma Wali, Thomas Middleton, Mariama Njie, and Jeanna Matthews. 2021. Gender Bias in Natural Language Processing Across Human Languages. In *Proceedings of the First Workshop on Trustworthy Natural Language Processing*. Association for Computational Linguistics (ACL), Online, 45–54. <https://doi.org/10.18653/v1/2021.TRUSTNLP-1.6>
  - [92] Rowan Hall Maudslay, Hila Gonen, Ryan Cotterell, and Simone Teufel. 2019. It’s All in the Name: Mitigating Gender Bias with Name-Based Counterfactual Data Substitution. In *EMNLP-IJCNLP 2019 - 2019 Conference on Empirical Methods in Natural Language Processing and 9th International Joint Conference on Natural Language Processing, Proceedings of the Conference*. Association for Computational Linguistics, 5267–5275. arXiv:1909.00871 <http://arxiv.org/abs/1909.00871>
  - [93] Chandler May, Alex Wang, Shikha Bordia, Samuel R. Bowman, and Rachel Rudinger. 2019. On Measuring Social Biases in Sentence Encoders. (mar 2019). arXiv:1903.10561 <http://arxiv.org/abs/1903.10561>
  - [94] Katherine McCurdy and Oguz Serbetci. 2020. Grammatical gender associations outweigh topical gender bias in crosslinguistic word embeddings. (may 2020). arXiv:2005.08864 <http://arxiv.org/abs/2005.08864>
  - [95] Ninareh Mehrabi, Thammie Gowda, Fred Morstatter, Nanyun Peng, and Aram Galstyan. 2019. Man is to Person as Woman is to Location: Measuring Gender Bias in Named Entity Recognition. (oct 2019). arXiv:1910.10872 <http://arxiv.org/abs/1910.10872>
  - [96] Josh Meyer, Lindy Rauchenstein, Joshua D. Eisenberg, and Nicholas Howell. 2020. Artie Bias Corpus: An Open Dataset for Detecting Demographic Bias in Speech Applications. In *Proceedings of the 12th Language Resources and Evaluation Conference*. European Language Resources Association (ELRA), Marseille, France, 6462–6468. <https://aclanthology.org/2020.lrec-1.796>
  - [97] Joshua R. Minot, Nicholas Cheney, Marc Maier, Danne C. Elbers, Christopher M. Danforth, and Peter Sheridan Dodds. 2021. *Interpretable bias mitigation for textual data: Reducing gender bias in patient notes while maintaining classification performance*. Technical Report. arXiv:2103.05841 <https://arxiv.org/abs/2103.05841v1>
  - [98] Inom Mirzaev, Anthony Schulte, Michael Conover, and Sam Shah. 2019. *Considerations for the Interpretation of Bias Measures of Word Embeddings*. Technical Report. arXiv:1906.08379 <http://arxiv.org/abs/1906.08379>
  - [99] Rodrigo Alejandro Chávez Mulca and Gerasimos Spanakis. 2020. Evaluating Bias In Dutch Word Embeddings. , 56–71 pages. <https://aclanthology.org/2020.gebnlp-1.6>
  - [100] Robert Munro and Alex (Carmen) Morrison. 2020. Detecting Independent Pronoun Bias with Partially-Synthetic Data Generation. In *Proceedings of the 2020 Conference on Empirical Methods in Natural Language Processing*. Association for Computational Linguistics (ACL), Online, 2011–2017. <https://doi.org/10.18653/v1/2020.EMNLP-MAIN.157>
  - [101] Moin Nadeem, Anna Bethke, and Siva Reddy. 2020. StereoSet: Measuring stereotypical bias in pretrained language models. (apr 2020). arXiv:2004.09456 <http://arxiv.org/abs/2004.09456>

- [102] Malvina Nissim, Rik van Noord, and Rob van der Goot. 2020. Fair is Better than Sensational: Man is to Doctor as Woman is to Doctor. *Computational Linguistics* (mar 2020), 1–11. [https://doi.org/10.1162/coli\\_a\\_00379](https://doi.org/10.1162/coli_a_00379) arXiv:1905.09866
- [103] Debora Nozza, Claudia Volpetti, and Elisabetta Fersini. 2019. Unintended Bias in Misogyny Detection. In *2019 IEEE/WIC/ACM International Conference on Web Intelligence (WI)*. 149–155.
- [104] Enoch Opanin Gyamfi, Yunbo Rao, Miao Gou, and Yanhua Shao. 2020. deb2viz: Debiasing gender in word embedding data using subspace visualization. In *Eleventh International Conference on Graphics and Image Processing (ICGIP 2019)*, Zhigeng Pan and Xun Wang (Eds.), Vol. 11373. SPIE, Hangzhou, China. <https://doi.org/10.1117/12.2557465>
- [105] Orestis Papakyriakopoulos, Simon Hegelich, Juan Carlos, Medina Serrano, and Fabienne Marco. 2020. Bias in Word Embeddings. (2020), 12. <https://doi.org/10.1145/3351095.3372843>
- [106] Ji Ho Park, Jamin Shin, and Pascale Fung. 2018. Reducing Gender Bias in Abusive Language Detection. *Proceedings of the 2018 Conference on Empirical Methods in Natural Language Processing, EMNLP 2018* (aug 2018), 2799–2804. arXiv:1808.07231 <http://arxiv.org/abs/1808.07231>
- [107] Radomir Popović, Florian Lemmerich, and Markus Strohmaier. 2020. Joint Multiclass Debiasing of Word Embeddings. (mar 2020). arXiv:2003.11520 <http://arxiv.org/abs/2003.11520>
- [108] Marcelo O. R. Prates, Pedro H. Avelar, and Luís C. Lamb. 2019. Assessing gender bias in machine translation: a case study with Google Translate. *Neural Computing and Applications* (mar 2019), 1–19. <https://doi.org/10.1007/s00521-019-04144-6>
- [109] Rasmus Précenth. 2019. *Word Embeddings and Gender Stereotypes in Swedish and English*. Master’s Thesis. Uppsala University.
- [110] Flavien Prost, Nithum Thain, and Tolga Bolukbasi. 2019. *Debiasing Embeddings for Reduced Gender Bias in Text Classification*. Technical Report. 69–75 pages. <https://github.com/tolga-b/debiaswe>
- [111] Arun K. Pujari, Ansh Mittal, Anshuman Padhi, Anshul Jain, Mukesh Jadon, and Vikas Kumar. 2019. Debiasing gender biased hindi words with word-embedding. In *ACM International Conference Proceeding Series*. Association for Computing Machinery, 450–456. <https://doi.org/10.1145/3377713.3377792>
- [112] Yusu Qian, Urwa Muaz, Ben Zhang, and Jae Won Hyun. 2019. Reducing Gender Bias in Word-Level Language Models with a Gender-Equalizing Loss Function. *ACL 2019 - 57th Annual Meeting of the Association for Computational Linguistics, Proceedings of the Student Research Workshop* (may 2019), 223–228. arXiv:1905.12801 <http://arxiv.org/abs/1905.12801>
- [113] Krithika Ramesh, Gauri Gupta, and Sanjay Singh. 2021. Evaluating Gender Bias in Hindi-English Machine Translation. In *Proceedings of the 3rd Workshop on Gender Bias in Natural Language Processing*. Association for Computational Linguistics (ACL), Online, 16–23. <https://doi.org/10.18653/V1/2021.GEBNLP-1.3>
- [114] Prashanth Rao and Maite Taboada. 2021. Gender Bias in the News: A Scalable Topic Modelling and Visualization Framework. *Frontiers in Artificial Intelligence* 4 (jun 2021). <https://doi.org/10.3389/FRAI.2021.664737/FULL>
- [115] Shauli Ravfogel, Yanai Elazar, Hila Gonen, Michael Twiton, and Yoav Goldberg. 2020. Null It Out: Guarding Protected Attributes by Iterative Nullspace Projection. (apr 2020). arXiv:2004.07667 <http://arxiv.org/abs/2004.07667>
- [116] Alexey Romanov, Maria De-Arteaga, Hanna Wallach, Jennifer Chayes, Christian Borgs, Alexandra Chouldechova, Sahin Geyik, Krishnamurthy Kenthapadi, Anna Rumshisky, and Adam Tauman Kalai. 2019. What’s in a Name? Reducing Bias in Bios without Access to Protected Attributes. (apr 2019). arXiv:1904.05233 <http://arxiv.org/abs/1904.05233>
- [117] Candace Ross, Boris Katz, and Andrei Barbu. 2020. Measuring Social Biases in Grounded Vision and Language Embeddings. (feb 2020). arXiv:2002.08911 <http://arxiv.org/abs/2002.08911>
- [118] David Rozado. 2020. Wide range screening of algorithmic bias in word embedding models using large sentiment lexicons reveals underreported bias types. *PLOS ONE* 15, 4 (apr 2020), e0231189. <https://doi.org/10.1371/journal.pone.0231189>
- [119] Rachel Rudinger, Chandler May, and Benjamin Van Durme. 2017. *Social Bias in Elicited Natural Language Inferences*. Technical Report. 74–79 pages. <https://github.com/cjmay/snli-ethics>
- [120] Rachel Rudinger, Jason Naradowsky, Brian Leonard, and Benjamin Van Durme. 2018. Gender Bias in Coreference Resolution. *NAACL HLT 2018 - 2018 Conference of the North American Chapter of the Association for Computational Linguistics: Human Language Technologies - Proceedings of the Conference 2* (apr 2018), 8–14. arXiv:1804.09301 <http://arxiv.org/abs/1804.09301>
- [121] Magnus Sahlgren and Fredrik Olsson. 2019. Gender Bias in Pretrained Swedish Embeddings. In *Proceedings of the 22nd Nordic Conference on Computational Linguistics*. Linköping University Electronic Press, Sweden, Turku, Finland, 35–43. <https://aclanthology.org/W19-6104>
- [122] Brenda Salenave Santana, Vinicius Woloszyn, and Leandro Krug Wives. 2018. Is there Gender bias and stereotype in Portuguese Word Embeddings?. In *International Conference on the Computational Processing of Portuguese*. arXiv:1810.04528 <http://arxiv.org/abs/1810.04528>
- [123] Maarten Sap, Saadia Gabriel, Lianhui Qin, Dan Jurafsky, Noah A. Smith, and Yejin Choi. 2020. Social Bias Frames: Reasoning about Social and Power Implications of Language. In *Proceedings of the 58th Annual Meeting of the Association for Computational Linguistics*. Association for Computational Linguistics, Online, 5477–5490. <https://doi.org/10.18653/v1/2020.acl-main.486> arXiv:1911.03891
- [124] Danielle Saunders and Bill Byrne. 2020. Reducing Gender Bias in Neural Machine Translation as a Domain Adaptation Problem. (apr 2020). arXiv:2004.04498 <http://arxiv.org/abs/2004.04498>
- [125] Beatrice Savoldi, Marco Gaido, Luisa Bentivogli, Matteo Negri, and Marco Turchi. 2021. Gender Bias in Machine Translation. *Transactions of the Association for Computational Linguistics* 9 (aug 2021), 845–874. [https://doi.org/10.1162/TACL\\_A\\_00401](https://doi.org/10.1162/TACL_A_00401) arXiv:2104.06001
- [126] Ramit Sawhney, Arshiya Aggarwal, and Rajiv Shah. 2021. An Empirical Investigation of Bias in the Multimodal Analysis of Financial Earnings Calls. In *Proceedings of the 2021 Conference of the North American Chapter of the Association for Computational Linguistics: Human Language Technologies*.

- Association for Computational Linguistics (ACL), Online, 3751–3757. <https://doi.org/10.18653/V1/2021.NAACL-MAIN.294>
- [127] Katja Geertruida Schmah, Tom Julian Viering, Stavros Makrodimitis, Arman Naseri Jahfari, David Tax, and Marco Loog. 2020. *Is Wikipedia succeeding in reducing gender bias? Assessing changes in gender bias in Wikipedia using word embeddings*. Technical Report. TU Delft. 94–103 pages. <https://doi.org/10.18653/v1/2020.nlpccs-1.11>
  - [128] João Sedoc and Lyle Ungar. 2019. *The Role of Protected Class Word Lists in Bias Identification of Contextualized Word Representations*. Technical Report. 55–61 pages. <https://github.com/jsedoc/>
  - [129] Procheta Sen and Debasis Ganguly. 2020. *Towards Socially Responsible AI: Cognitive Bias-Aware Multi-Objective Learning*. Technical Report. <https://ojs.aaai.org/index.php/AAAI/article/view/5654>
  - [130] Sima Sharifirad, Alon Jacovi, and Stan Matwin. 2019. Learning and Understanding Different Categories of Sexism Using Convolutional Neural Network’s Filters. In *Proceedings of the 2019 Workshop on Widening NLP*. 21–23. <https://doi.org/10.1177/1741659016652445>
  - [131] Sima Sharifirad and Stan Matwin. 2019. Using Attention-based Bidirectional LSTM to Identify Different Categories of Offensive Language Directed Toward Female Celebrities. In *Proceedings of the 2019 Workshop on Widening NLP*. Association for Computational Linguistics, Florence, Italy, 46–48. <https://aclanthology.org/W19-3616>
  - [132] Shanya Sharma, Manan Dey, and Koustuv Sinha. 2020. Evaluating Gender Bias in Natural Language Inference. In *NeurIPS 2020 Workshop on Dataset Curation and Security*. arXiv:2105.05541 <https://arxiv.org/abs/2105.05541v1>
  - [133] Judy Hanwen Shen, Lauren Fratamico, Iyad Rahwan, and Alexander M Rush. 2018. *Darling or Babygirl? Investigating Stylistic Bias in Sentiment Analysis*. Technical Report. <http://textblob.readthedocs.io/en/dev/>
  - [134] Emily Sheng, Kai-Wei Chang, Premkumar Natarajan, and Nanyun Peng. 2019. The Woman Worked as a Babysitter: On Biases in Language Generation. *EMNLP-IJCNLP 2019 - 2019 Conference on Empirical Methods in Natural Language Processing and 9th International Joint Conference on Natural Language Processing, Proceedings of the Conference (sep 2019)*, 3407–3412. arXiv:1909.01326 <http://arxiv.org/abs/1909.01326>
  - [135] Emily Sheng, Kai-Wei Chang, Premkumar Natarajan, and Nanyun Peng. 2020. Towards Controllable Biases in Language Generation. (may 2020). arXiv:2005.00268 <http://arxiv.org/abs/2005.00268>
  - [136] Eli Sherman, Keith Harrigan, Carlos Aguirre, and Mark Dredze. 2021. Towards Understanding the Role of Gender in Deploying Social Media-Based Mental Health Surveillance Models. In *Proceedings of the Seventh Workshop on Computational Linguistics and Clinical Psychology: Improving Access*. Association for Computational Linguistics (ACL), Online, 217–223. <https://doi.org/10.18653/V1/2021.CLPSYCH-1.23>
  - [137] Seungjae Shin, Kyungwoo Song, JoonHo Jang, Hyemi Kim, Weonyoung Joo, and Il-Chul Moon. 2020. Neutralizing Gender Bias in Word Embedding with Latent Disentanglement and Counterfactual Generation. (apr 2020). arXiv:2004.03133 <http://arxiv.org/abs/2004.03133>
  - [138] Andrew Silva, Pradyumna Tambwekar, and Matthew Gombolay. 2021. Towards a Comprehensive Understanding and Accurate Evaluation of Societal Biases in Pre-Trained Transformers. In *Proceedings of the 2021 Conference of the North American Chapter of the Association for Computational Linguistics: Human Language Technologies*. Association for Computational Linguistics (ACL), Online, 2383–2389. <https://doi.org/10.18653/V1/2021.NAACL-MAIN.189>
  - [139] Gabriel Stanovsky, Noah A. Smith, and Luke Zettlemoyer. 2019. Evaluating Gender Bias in Machine Translation. *ACL 2019 - 57th Annual Meeting of the Association for Computational Linguistics, Proceedings of the Conference (jun 2019)*, 1679–1684. arXiv:1906.00591 <http://arxiv.org/abs/1906.00591>
  - [140] Tony Sun, Andrew Gaut, Shirlyn Tang, Yuxin Huang, Mai ElSherief, Jieyu Zhao, Diba Mirza, Elizabeth Belding, Kai-Wei Chang, and William Yang Wang. 2019. Mitigating Gender Bias in Natural Language Processing: Literature Review. In *ACL 2019 - 57th Annual Meeting of the Association for Computational Linguistics, Proceedings of the Conference*. Association for Computational Linguistics (ACL), Florence, Italy, 1630–1640. arXiv:1906.08976 <http://arxiv.org/abs/1906.08976>
  - [141] Adam Sutton, Thomas Lansdall-Welfare, and Nello Cristianini. 2018. Biased Embeddings from Wild Data: Measuring, Understanding and Removing. *Lecture Notes in Computer Science (including subseries Lecture Notes in Artificial Intelligence and Lecture Notes in Bioinformatics)* 11191 LNCS (jun 2018), 328–339. arXiv:1806.06301 <http://arxiv.org/abs/1806.06301>
  - [142] Chris Sweeney and Maryam Najafian. 2020. Reducing Sentiment Polarity for Demographic Attributes in Word Embeddings using Adversarial Learning. (2020). <https://doi.org/10.1145/3351095.3372837>
  - [143] Nathaniel Swinger, Maria De-Arteaga, Neil Thomas Heffernan IV, Mark DM Leiserson, and Adam Tauman Kalai. 2019. What are the Biases in My Word Embedding?. In *Artificial Intelligence, Ethics, and Society*. Association for Computing Machinery, New York, NY, USA, 305–311. <https://doi.org/10.1145/3306618.3314270>
  - [144] Masashi Takeshita, Yuki Katsumata, Rafal Rzepka, and Kenji Araki. 2020. Can Existing Methods Debias Languages Other than English? First Attempt to Analyze and Mitigate Japanese Word Embeddings. In *Proceedings of the Second Workshop on Gender Bias in Natural Language Processing*. Association for Computational Linguistics, Barcelona, Spain (Online), 44–55. <https://aclanthology.org/2020.gebnlp-1.5>
  - [145] Yi Chern Tan and L Elisa Celis. 2019. *Assessing Social and Intersectional Biases in Contextualized Word Representations*. Technical Report. 13230–13241 pages. <https://github.com/openai/gpt-2-output-dataset>
  - [146] Mike Thelwall. 2018. Gender bias in sentiment analysis. *Online Information Review* 42, 1 (2018), 45–57. <https://doi.org/10.1108/OIR-05-2017-0139>
  - [147] Samia Touileb, Lilja Øvrelid, and Erik Velldal. 2021. Using Gender- and Polarity-Informed Models to Investigate Bias. In *Proceedings of the 3rd Workshop on Gender Bias in Natural Language Processing*. Association for Computational Linguistics (ACL), Online, 66–74. <https://doi.org/10.18653/V1/2021.GEBNLP-1.8>
  - [148] Ameya Vaidya, Feng Mai, and Yue Ning. 2019. Empirical Analysis of Multi-Task Learning for Reducing Model Bias in Toxic Comment Detection. (sep 2019). arXiv:1909.09758 <http://arxiv.org/abs/1909.09758>

- [149] Eva Vanmassenhove, Christian Hardmeier, and Andy Way. 2019. Getting Gender Right in Neural Machine Translation. *Proceedings of the 2018 Conference on Empirical Methods in Natural Language Processing, EMNLP 2018* (sep 2019), 3003–3008. <https://doi.org/10.18653/v1/D18-1334> arXiv:1909.05088
- [150] Eva Vanmassenhove, Dimitar Shterionov, and Matthew Gwilliam. 2021. Machine Translationese: Effects of Algorithmic Bias on Linguistic Complexity in Machine Translation. , 2203–2213 pages. <https://aclanthology.org/2021.eacl-main.188>
- [151] Jesse Vig, Sebastian Gehrmann, Yonatan Belinkov, Sharon Qian, Daniel Nevo, Yaron Singer, and Stuart Shieber. 2020. Causal Mediation Analysis for Interpreting Neural NLP: The Case of Gender Bias. (apr 2020). arXiv:2004.12265 <http://arxiv.org/abs/2004.12265>
- [152] Jesse Vig, Sebastian Gehrmann, Yonatan Belinkov, Sharon Qian, Daniel Nevo, Yaron Singer, and Stuart Shieber. 2020. Investigating Gender Bias in Language Models Using Causal Mediation Analysis. In *34th Conference on Neural Information Processing Systems (NeurIPS 2020)*. NeurIPS, Vancouver, Canada, 14 pages. [https://www.cs.technion.ac.il/~sim\\$belinkov/assets/pdf/neurips2020.pdf](https://www.cs.technion.ac.il/~sim$belinkov/assets/pdf/neurips2020.pdf)
- [153] Tianlu Wang, Xi Victoria Lin, Nazneen Fatema Rajani, Bryan McCann, Vicente Ordonez, and Caiming Xiong. 2020. Double-Hard Debias: Tailoring Word Embeddings for Gender Bias Mitigation. (may 2020), 5443–5453. arXiv:2005.00965 <http://arxiv.org/abs/2005.00965>
- [154] Tianlu Wang, Xi Victoria Lin, Nazneen Fatema Rajani, Bryan McCann, Vicente Ordonez, and Caiming Xiong. 2021. [RE] Double-Hard Debias: Tailoring Word Embeddings for Gender Bias Mitigation. (apr 2021), 5443–5453. <https://doi.org/10.18653/v1/2020.acl-main.484> arXiv:2104.06973
- [155] Zili Wang. 2019. *MSnet: A BERT-based Network for Gendered Pronoun Resolution*. Technical Report. 89–95 pages. <https://github.com/google-research->
- [156] Kellie Webster, Marta R Costa-Jussà, Christian Hardmeier, and Will Radford. 2019. *Gendered Ambiguous Pronouns (GAP) Shared Task at the Gender Bias in NLP Workshop 2019*. Technical Report. 1–7 pages. <https://www.kaggle.com/c/>
- [157] Kellie Webster, Marta Recasens, Vera Axelrod, and Jason Baldridge. 2018. Mind the GAP: A Balanced Corpus of Gendered Ambiguous Pronouns. *Transactions of the Association for Computational Linguistics* 6 (dec 2018), 605–617. [https://doi.org/10.1162/tacl\\_a\\_00240](https://doi.org/10.1162/tacl_a_00240) arXiv:1810.05201
- [158] Austin P. Wright, Omar Shaikh, Haekyu Park, Will Epperson, Muhammed Ahmed, Stephane Pinel, Diyi Yang, Duen Horng, and Chau. 2020. RECAST: Interactive Auditing of Automatic Toxicity Detection Models. (jan 2020). arXiv:2001.01819 <http://arxiv.org/abs/2001.01819>
- [159] Yinchuan Xu and Junlin Yang. 2019. Look Again at the Syntax: Relational Graph Convolutional Network for Gendered Ambiguous Pronoun Resolution. In *Proceedings of the 1st Workshop on Gender Bias in Natural Language Processing*. Association for Computational Linguistics, Florence, Italy, 96–101. <https://www.aclweb.org/anthology/W19-3814/>
- [160] Kai-Chou Yang, Timothy Niven, Tzu-Hsuan Chou, and Hung-Yu Kao. 2019. Fill the GAP: Exploiting BERT for Pronoun Resolution. In *Proceedings of the 1st Workshop on Gender Bias in Natural Language Processing*. Association for Computational Linguistics, Florence, Italy, 102–106. <https://www.aclweb.org/anthology/W19-3815/>
- [161] Zekun Yang and Juan Feng. 2020. A Causal Inference Method for Reducing Gender Bias in Word Embedding Relations. In *Proceedings of the AAAI Conference on Artificial Intelligence*, Vol. 34. AAAI press, New York, NY, USA, 9434–9441. <https://doi.org/10.1609/AAAI.V34I05.6486> arXiv:1911.10787
- [162] Catherine Yeo and Alyssa Chen. 2020. Defining and Evaluating Fair Natural Language Generation. In *Proceedings of the The Fourth Widening Natural Language Processing Workshop at ACL*. Association for Computational Linguistics, Seattle, USA, 107–109. <https://doi.org/10.18653/v1/2020.winlp-1.27> arXiv:2008.01548
- [163] Brian Hu Zhang, Blake Lemoine, and Margaret Mitchell. 2018. Mitigating Unwanted Biases with Adversarial Learning. In *AIES 2018 - Proceedings of the 2018 AAAI/ACM Conference on AI, Ethics, and Society*. Association for Computing Machinery, Inc, 335–340. <https://doi.org/10.1145/3278721.3278779> arXiv:1801.07593
- [164] Chong Zhang, Jieyu Zhao, Huan Zhang, Kai-Wei Chang, and Cho-Jui Hsieh. 2021. Double Perturbation: On the Robustness of Robustness and Counterfactual Bias Evaluation. In *Proceedings of the 2021 Conference of the North American Chapter of the Association for Computational Linguistics: Human Language Technologies*. Association for Computational Linguistics (ACL), Online, 3899–3916. <https://doi.org/10.18653/V1/2021.NAACL-MAIN.305>
- [165] Guanhua Zhang, Bing Bai, Junqi Zhang, Kun Bai, Conghui Zhu, and Tiejun Zhao. 2020. Demographics Should Not Be the Reason of Toxicity: Mitigating Discrimination in Text Classifications with Instance Weighting. In *Proceedings of the 58th Annual Meeting of the Association for Computational Linguistics*. Association for Computational Linguistics, Online, 4134–4145. <https://doi.org/10.18653/v1/2020.acl-main.380>
- [166] Haoran Zhang, Amy X. Lu, Mohamed Abdalla, Matthew McDermott, and Marzyeh Ghassemi. 2020. Hurtful words: Quantifying Biases in Clinical Contextual Word Embeddings. In *ACM CHIL 2020 - Proceedings of the 2020 ACM Conference on Health, Inference, and Learning*. Association for Computing Machinery, Inc, 110–120. <https://doi.org/10.1145/3368555.3384448>
- [167] Jieyu Zhao and Kai-Wei Chang. 2020. LOGAN: Local Group Bias Detection by Clustering. In *Proceedings of the 2020 Conference on Empirical Methods in Natural Language Processing*. Association for Computational Linguistics (ACL), 1968–1977. <https://doi.org/10.18653/v1/2020.emnlp-main.155> arXiv:2010.02867
- [168] Jieyu Zhao, Subhabrata Mukherjee, Saghar Hosseini, Kai-Wei Chang, and Ahmed Hassan Awadallah. 2020. Gender Bias in Multilingual Embeddings and Cross-Lingual Transfer. (may 2020), 2896–2907. arXiv:2005.00699 <http://arxiv.org/abs/2005.00699>
- [169] Jieyu Zhao, Tianlu Wang, Mark Yatskar, Ryan Cotterell, Vicente Ordonez, and Kai-Wei Chang. 2019. Gender Bias in Contextualized Word Embeddings. In *NAACL HLT 2019 - 2019 Conference of the North American Chapter of the Association for Computational Linguistics: Human Language Technologies - Proceedings of the Conference*, Vol. 1. Association for Computational Linguistics (ACL), Minneapolis, Minnesota, 629–634. <https://doi.org/10.18653/V1/N19-1064>

- [170] Jieyu Zhao, Tianlu Wang, Mark Yatskar, Ryan Cotterell, Vicente Ordonez, and Kai-Wei Chang. 2019. Gender Bias in Contextualized Word Embeddings. *NAACL HLT 2019 - 2019 Conference of the North American Chapter of the Association for Computational Linguistics: Human Language Technologies - Proceedings of the Conference 1* (apr 2019), 629–634. arXiv:1904.03310 <http://arxiv.org/abs/1904.03310>
- [171] Jieyu Zhao, Tianlu Wang, Mark Yatskar, Vicente Ordonez, and Kai-Wei Chang. 2017. Men Also Like Shopping: Reducing Gender Bias Amplification using Corpus-level Constraints. *EMNLP 2017 - Conference on Empirical Methods in Natural Language Processing, Proceedings* (jul 2017), 2979–2989. arXiv:1707.09457 <http://arxiv.org/abs/1707.09457>
- [172] Jieyu Zhao, Tianlu Wang, Mark Yatskar, Vicente Ordonez, and Kai-Wei Chang. 2018. Gender Bias in Coreference Resolution: Evaluation and Debiasing Methods. *NAACL HLT 2018 - 2018 Conference of the North American Chapter of the Association for Computational Linguistics: Human Language Technologies - Proceedings of the Conference 2* (apr 2018), 15–20. arXiv:1804.06876 <http://arxiv.org/abs/1804.06876>
- [173] Jieyu Zhao, Yichao Zhou, Zeyu Li, Wei Wang, and Kai-Wei Chang. 2018. Learning Gender-Neutral Word Embeddings. In *Proceedings of the 2018 Conference on Empirical Methods in Natural Language Processing*. Association for Computational Linguistics, Brussels, Belgium, 4847–4853. <https://doi.org/10.18653/v1/D18-1521>
- [174] Pei Zhou, Weijia Shi, Jieyu Zhao, Kuan-Hao Huang, Muhao Chen, Ryan Cotterell, and Kai-Wei Chang. 2019. Examining Gender Bias in Languages with Grammatical Gender. In *EMNLP-IJCNLP 2019 - 2019 Conference on Empirical Methods in Natural Language Processing and 9th International Joint Conference on Natural Language Processing, Proceedings of the Conference*. Association for Computational Linguistics, Hong Kong, 5276–5284. arXiv:1909.02224 <http://arxiv.org/abs/1909.02224>
- [175] Ran Zmigrod, Sabrina J. Mielke, Hanna Wallach, and Ryan Cotterell. 2019. Counterfactual Data Augmentation for Mitigating Gender Stereotypes in Languages with Rich Morphology. *ACL 2019 - 57th Annual Meeting of the Association for Computational Linguistics, Proceedings of the Conference* (jun 2019), 1651–1661. arXiv:1906.04571 <http://arxiv.org/abs/1906.04571>
